# Supplementary material for: Two Simple Principles for Diffusion-Based Test-Time Adaptation
Source: arXiv:2312.05274 source file (2025-03-12)
Supplement: Supplementary file 1 [file X_suppl.tex]

\clearpage
\appendix
\setcounter{page}{1}
\maketitlesupplementary

\section{Visualization}
To show the effectiveness of SEDA, we report the additional visualization results.

Figure.~\ref{fig:differentmodels} reports the visualization of SEDA compared with the target-to-source baselines. It was found that SEDA maintains semantics as much as possible. In contrast to corruption, SEDA can recover part of the semantics. Meanwhile, in spatter corruption, SEDA can remove the extra noise and keep the label semantic, which proves its effectiveness. Meanwhile, we also report the ablation study about the sampling strategy. It could be found that the sampling strategy could improve the quality of the generated image, proving the sampling strategy's necessity. Meanwhile, it also shows that the sampling strategy is important for the acceleration method in target-to-source methods, which is an additional finding in our work.

\textbf{Hyperparameters.} SEDA contains two hyperparameters: the special time $t$ for $g^1$ and the small weight $\eta$ for $g^2$. We report the influence of the hyperparameters on the quality of the generated images shown in Figure.~\ref{fig:abationstudy_time} and Figure.~\ref{fig:abationstudy_theta}, respectively. For special time $t$, previous works~\cite{Zecon,Diffuse} show that the diffusion model will focus on the local details when the $t$ tends to be $0$. However, the corruption's extra noise, such as the impulse noise, will influence the generated images if we directly set $t=0$. In this condition, we slightly increase the $t$ to let the diffusion model focus on the local details and ignore part of the noise. As shown in Figure.~\ref{fig:abationstudy_time}, when $t=0.1$, the diffusion model starts to drop the local detail since it can be found that the quality of the generated image against contrast is decreasing. In internal $t\in[0.05,0.008]$, the generated images are high quality compared with the interval $t\in[0.007,0.005]$. Therefore, choosing the value in internal $[0.05,0.008]$ can get a great result. In our work, we directly set $t=0.008$.

We also report the influence of $\eta$ shown in Figure.~\ref{fig:abationstudy_theta}. Firstly, it can be found that it is necessary to use the $f^2$ to keep the overall style. When $\eta =0$, the generated images have low quality. By increasing the $\eta$ slightly, the image quality will increase. However, with the increasing of the $\eta$, the defect of the MSE will introduce extra noise since corruption will break the label semantic and negatively influence the generated images. In this condition, we just set $\eta in [0.01,0.03]$ interval to avoid introducing too much corruption, whereas, in our work, we use $\eta=0.02$.

\begin{figure*}[h!]
    \centering
    \includegraphics[width=\textwidth]{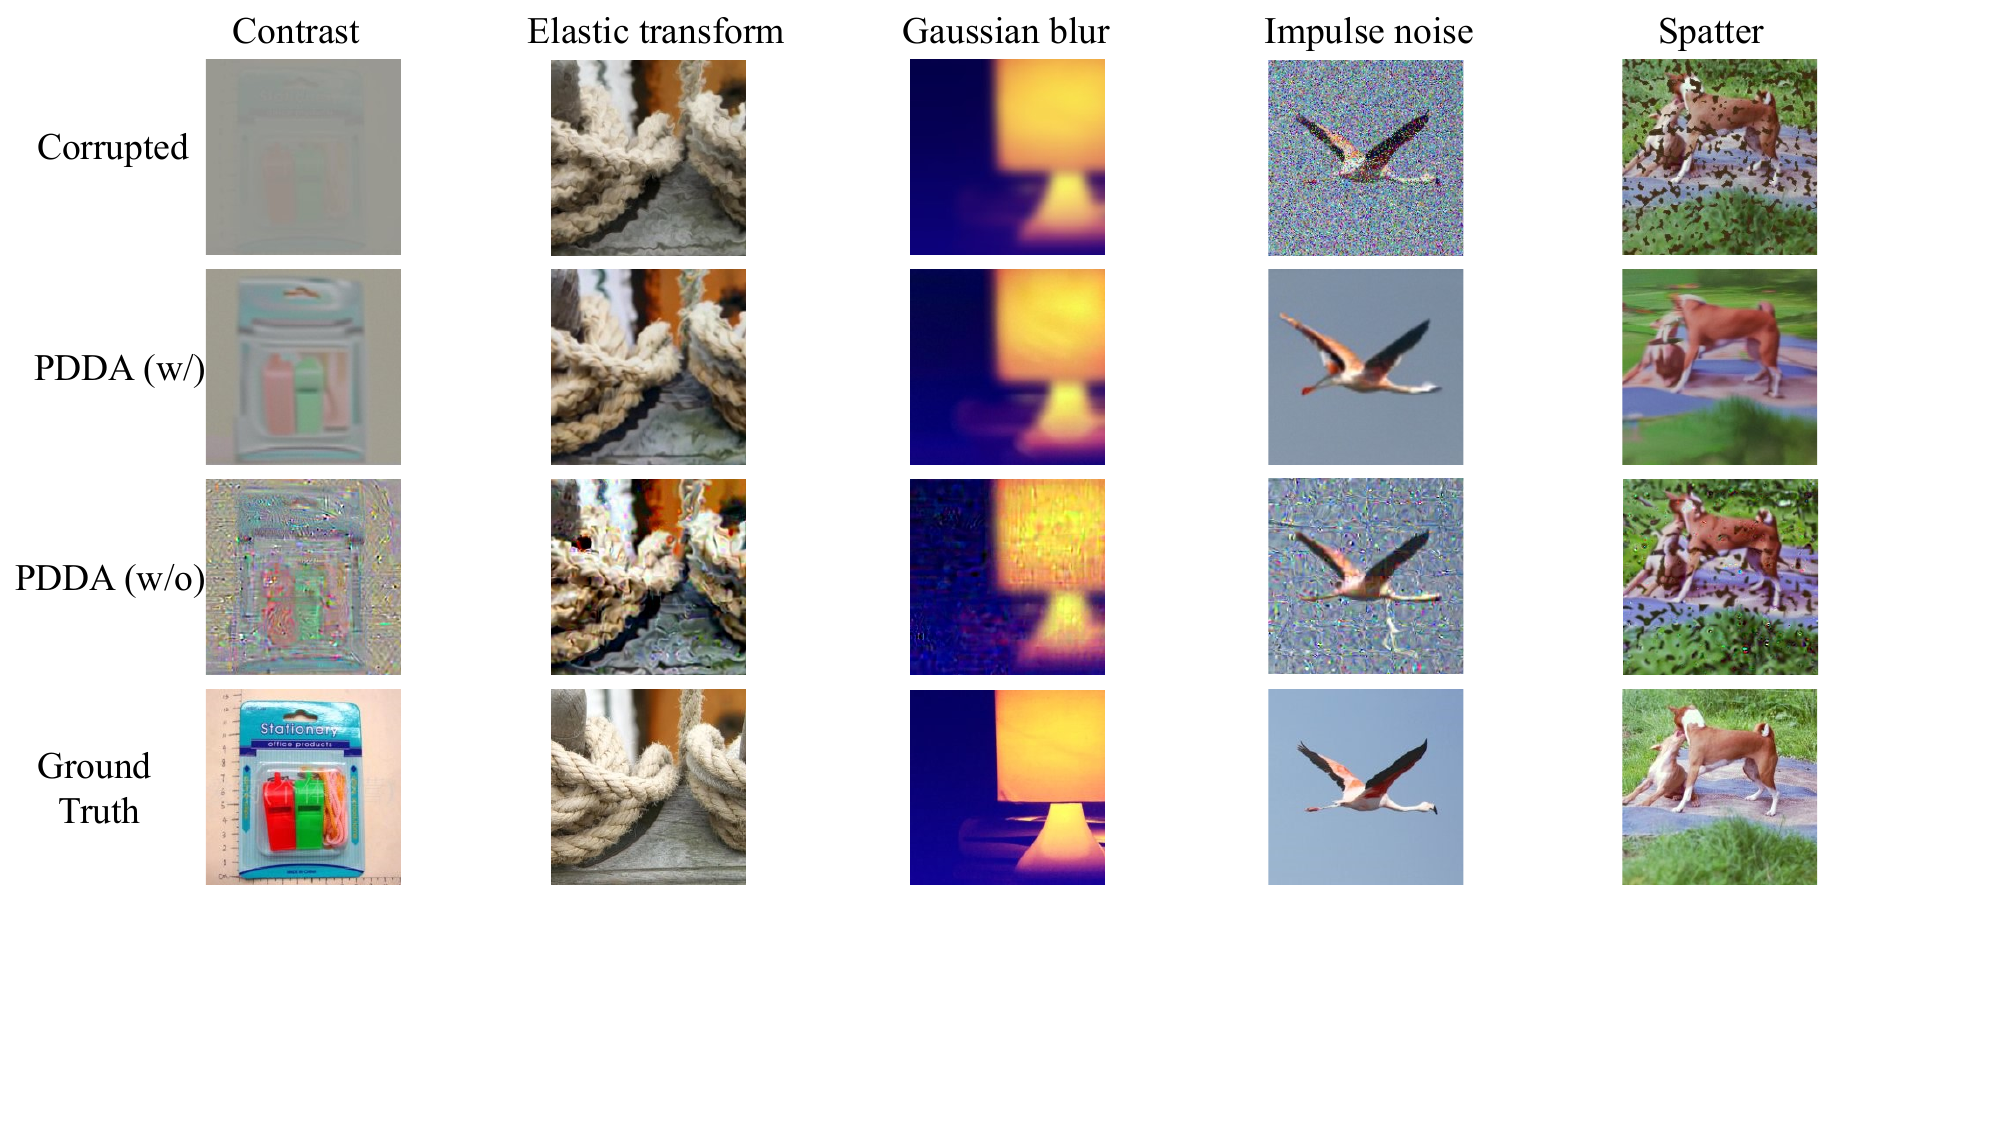}
    \caption{Visualization of ablation study for different models against different corruption, where our (no sampling) means we do not use the proposed sampling strategy and ground truth is the image without corruption.} 
    \label{fig:differentmodels}
\end{figure*}
\begin{figure*}[h!]
    \centering
    \includegraphics[width=\textwidth]{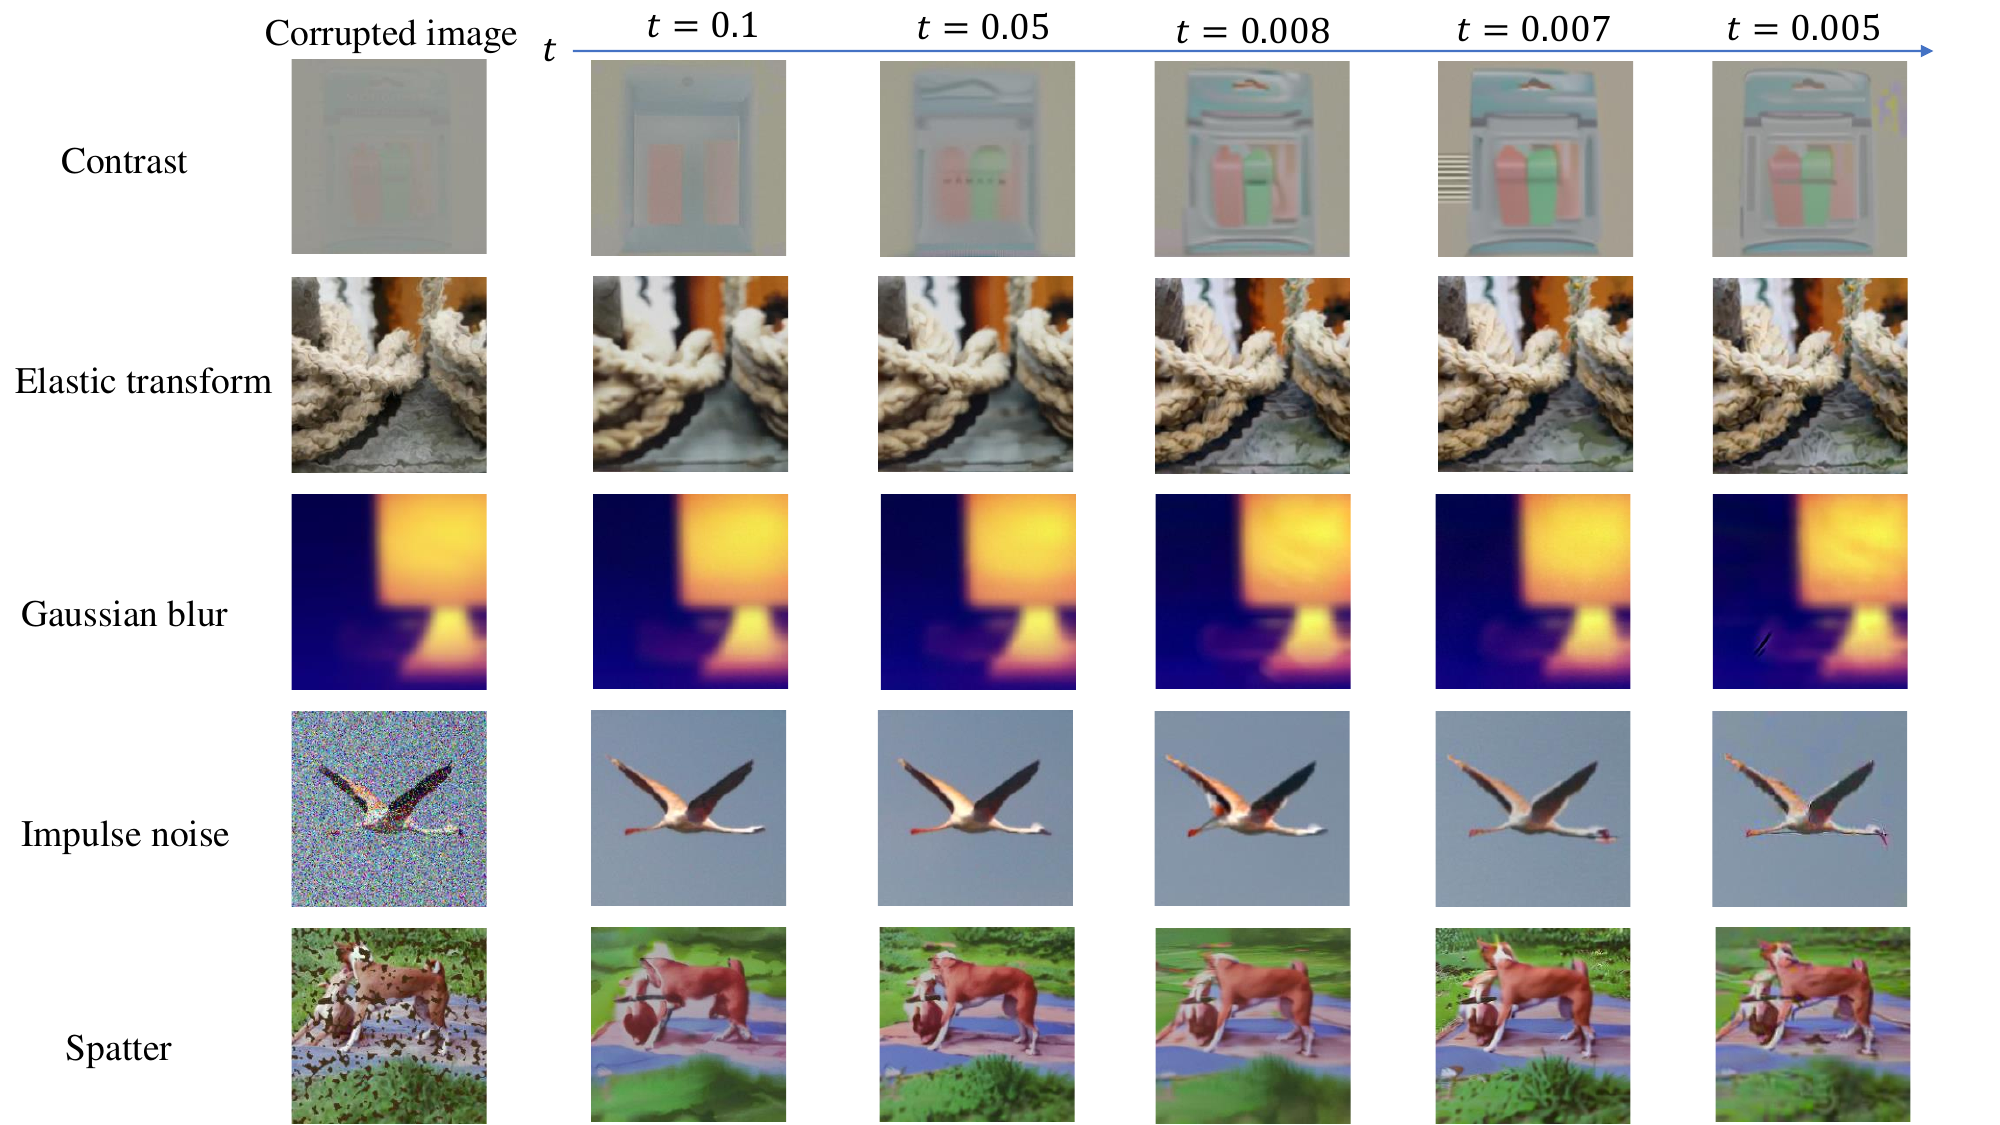}
    \caption{Visualization of ablation study for $t$ in $f^1$ against different corruption.} 
    \label{fig:abationstudy_time}
\end{figure*}
\begin{figure*}[h!]
    \centering
    \includegraphics[width=\textwidth]{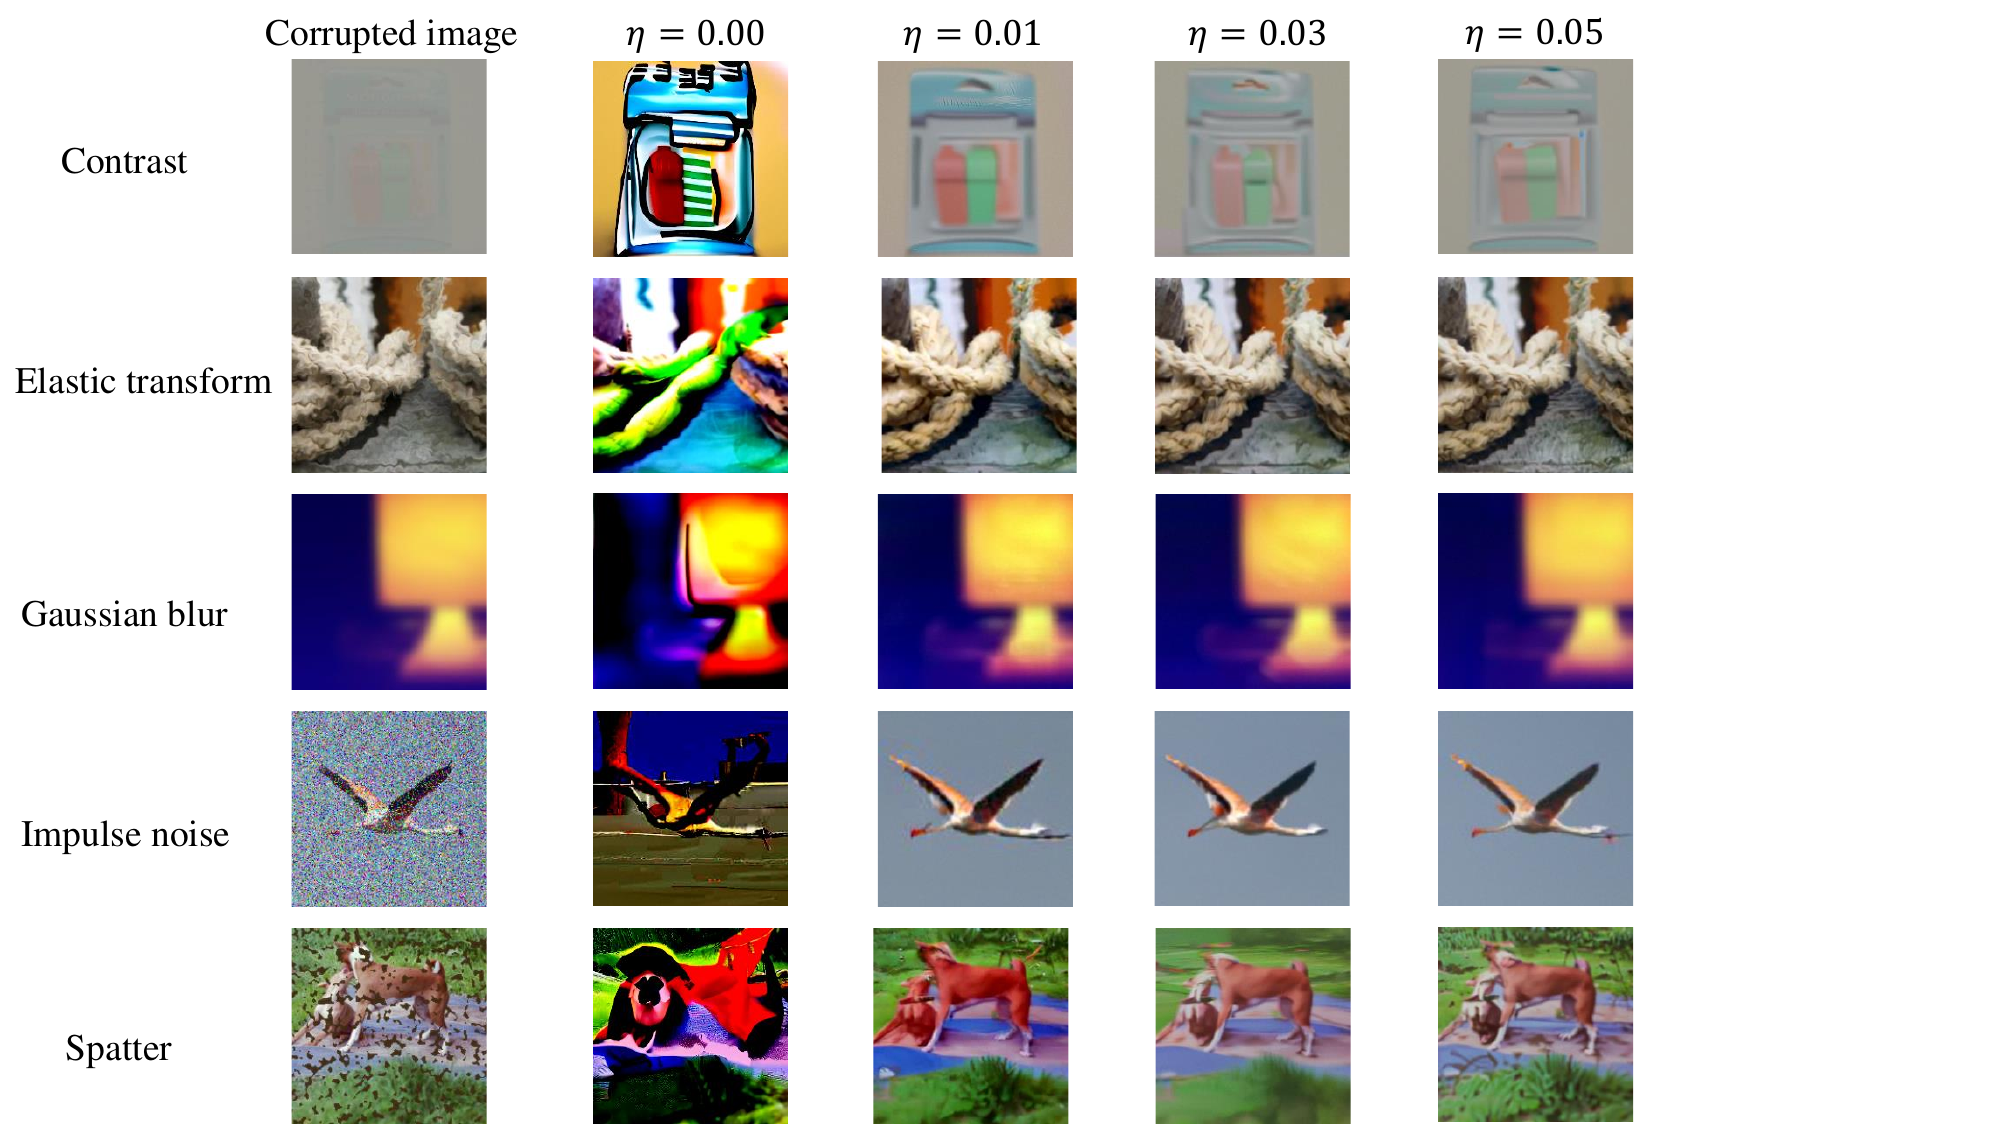}
    \caption{Visualization of ablation study for $\eta$ in $f^2$ against different corruption.} 
    \label{fig:abationstudy_theta}
\end{figure*}

 \begin{table*}
    \centering
    \caption{Classification accuracy(\%) against the different types of corruption on CIFAR-10C under ResNet-26, where Gaussian-B is the Gaussian blur corruption, and Gaussian-N is the Gaussian noise.}
    \begin{adjustbox}{width={\textwidth},totalheight={\textheight},keepaspectratio}
   \setlength{\tabcolsep}{2px}{
    \begin{tabular}{c c c c c c c c c c c c c c c c c c c c c}
        \toprule
        \textbf{Method} & \scriptsize  \textbf{Brightness} & \scriptsize \textbf{Contrast} & \scriptsize \textbf{Defocus} & \scriptsize \textbf{Elastic} & \scriptsize \textbf{Fog}& \scriptsize \textbf{Frost}& \scriptsize\textbf{Gaussian-B}& \scriptsize \textbf{Gaussian-N}&\scriptsize \textbf{Glass}& \scriptsize \textbf{Impulse}& \scriptsize \textbf{JPEG}& \scriptsize \textbf{Motion}& \scriptsize \textbf{Pixel}& \scriptsize \textbf{Saturate}& \scriptsize \textbf{Shot}&\scriptsize \textbf{Snow}&\scriptsize \textbf{Spatter}&\scriptsize \textbf{Speckle}&\scriptsize \textbf{Zoom}&\scriptsize \textbf{Avg.}  \\
        \midrule
        \textbf{Source-to-target}\\
        \midrule
        MEMO~\cite{MEMO} & 88.73& 82.03& 86.16& 79.46& 82.81& 75.45& 79.13& 63.84& 52.46& 54.91& 65.85& 70.54& 60.94& 66.52& 49.89& 47.99& 47.66& 37.95& 40.29& 64.87 \\
        TENT~\cite{Tent} & 86.98& \textbf{83.85} & \textbf{86.46}& 80.47& \textbf{83.33}& 82.03& \textbf{82.03}& 70.57& \textbf{70.05}& 72.14& 77.08& \textbf{83.85}& 78.91& 85.94& 75.52& 76.3& 80.99& 77.6& \textbf{84.64}& 79.93   \\
        \midrule
        \textbf{Target-to-source} \\
        \midrule
        DiffPure~\cite{DiffurePure} &  77.5& 62.29& 64.17& 61.88& 70.42& 57.71& 56.67& 46.25& 40.42& 52.71& 61.46& 57.29& 61.04& 75.63& 52.92& 65.0& 67.92& 55.83& 57.5& 60.24\\
        BackToSource~\cite{BacktoSource}& 88.4& 63.2& 75.2& 76.8& 82.4& 74.2& 68.0& 73.0& 64.4& 75.2& 78.8& 71.2& 81.0& 84.0& 76.4& 72.4& 80.8& 79.4& 67.2& 75.37 \\
        SEDA (Our) & \textbf{89.2}& 68.44& \textbf{77.2}& 75.33& 80.0& \textbf{84.4}& 70.4& \textbf{83.78}& 68.0 & \textbf{84.89}& \textbf{83.33}& 71.4& \textbf{79.2}& \textbf{87.8}& \textbf{87.0}& \textbf{81.11}& \textbf{82.8}& \textbf{86.2}& 68.8& \textbf{79.96} \\ 
        \bottomrule
   \end{tabular}}
    \end{adjustbox} 
    \label{tab:cifar10c-resnet}
\end{table*}
